# Supplementary material for: Bias in Unsupervised Anomaly Detection in Brain MRI
Source: arXiv:2308.13861 source file (2023-08-26)
Supplement: Supplementary file 1 [file 3_3_appendix.tex]

% \begin{figure}
%     \centering
%     \includegraphics[width=0.9\columnwidth]{figures/fig_corr_age.png}
%     \caption{Correlation with age. The first two column show if the residual errors correlate with age on healthy and AD. It seems that age has a positive correlation with age for healthy, but no correlation for AD. The next three columns show if there are drifts between the age distributions between the i). healthy and AD of the target distribution; ii). Healthy-train vs. healthy-target; and iii). AD-train vs. AD-target. (Temporary placeholder -- will not make it to this submission.) }
%     \label{fig::corr_age}
% \end{figure}
